# Supplementary material for: SparCAssist: A Model Risk Assessment Assistant Based on Sparse Generated Counterfactuals
Source: arXiv:2205.01588 source file (2022-05-03)
Supplement: Supplementary file 1 [file appendix.tex]

\appendix
